# Supplementary material for: Appropriateness of Performance Indices for Imbalanced Data Classification: An Analysis
Source: arXiv:2008.11752 source file (2020-08-26)
Supplement: Supplementary file 1 [file suppli.tex]

\documentclass[3p]{myElsarticle}

\usepackage{graphicx}
\usepackage{amsmath}
\usepackage{amsthm}
\usepackage{amssymb}
\usepackage{amsfonts}
\usepackage[caption=false]{subfig}
\usepackage{threeparttable}
\usepackage{color}
\usepackage{array}
\usepackage{booktabs}
\usepackage{mathrsfs}
\usepackage{multirow}
\usepackage{url}

\newdefinition{definition}{Definition}
\newdefinition{assumption}{Assumption}
\newdefinition{condition}{Condition}
\newdefinition{remark}{Remark}

\newcolumntype{C}[1]{>{\centering\let\newline\\\arraybackslash\hspace{0pt}}m{#1}}
\newcolumntype{L}{>{\centering\arraybackslash}m{4cm}}

\begin{document}

\title{Appropriateness of Performance Indices for Imbalanced Data Classification: An Analysis \\ \textsc{Supplementary Material}}

\author[1]{Sankha Subhra Mullick}
\ead{sankha\_r@isical.ac.in}

\author[2]{Shounak Datta}
\ead{shounak.jaduniv@gmail.com}

\author[3]{Sourish Gunesh Dhekane}
\ead{sourishdhekane@gmail.com}

\author[1]{Swagatam Das\corref{cor1}}
\ead{swagatam.das@isical.ac.in}

%\author[4]{Bijaya Ketan Panigrahi}
%\ead{bkpanigrahi@ee.iitd.ac.in}

\cortext[cor1]{Corresponding author}

\address[1]{Electronics and Communication Sciences Unit, Indian Statistical Institute, Kolkata, India}
\address[2]{Department of Electrical and Computer Engineering, Duke University, Durham, NC, USA}
\address[3]{Department of Computer Science and Engineering, Indian Institute of Information Technology, Guwahati, India}
%\address[4]{Department of Electrical Engineering, Indian Institute of Technology, Delhi, India}

\maketitle

\section{Construction of datasets used in Example 1}
\subsection{Datasets used for illustration of Type 1 distortions}
For the two class datasets, both of the classes are sampled from $\mathcal{N}(\mu_{i}, \Sigma_{i})$, where $\mu_{i}$ and $\Sigma_{i}$ are respectively the mean and co-variance matrix of the $i^{th}$ class, and $i \in \{1, 2\}$. The parameters are as follows:
\begin{equation*}
    \mu_{1}=[3 \; 3]^{T} \; \text{and} \; \mu_{2}=[7.5 \; 3]^{T}.
\end{equation*}
\begin{equation*}
    \Sigma_{1}=
    \begin{bmatrix}
    0.45 & 0 \\
    0 & 0.45 \\
    \end{bmatrix} 
    \; \text{and} \;
    \begin{bmatrix}
    0.25 & 0 \\
    0 & 0.25 \\
    \end{bmatrix} 
\end{equation*}
We start with sampling 5000 data points from each class and then sub-sample from the one in the left to construct the datasets of gradually deteriorating behavior. 
\subsection{Datasets used for illustration of Type 2 distortions}
Similar to the ones used to construct the datasets used to illustrate the effect of Type 1 distortion in Example 1, here also the classes are sampled from $\mathcal{N}(\mu_{i}, \Sigma$), where $i \in \{1, 2, 3, 4, 5, 6\}$. For the $i^{th}$ class the center $\mu_{i}$, lies on the $i^{th}$ vertex of a regular hexagon centered at $[0 \; 0]^{T}$, with edge length of 5 unit. Therefore, 
\begin{equation*}
    \mu_{1}=[-2.5 \; -4.33]^{T}, \;
    \mu_{2}=[-5 \; 0]^{T}, \;
    \mu_{3}=[-2.5 \; 4.33]^{T}, \;
    \mu_{4}=[2.5 \; 4.33]^{T}, \;
    \mu_{5}=[5 \; 0]^{T}, \; 
    \mu_{6}=[2.5 \; -4.33]^{T}.
\end{equation*}
\begin{equation*}
    \Sigma=
    \begin{bmatrix}
    0.08 & 0 \\
    0 & 0.08 \\
    \end{bmatrix}
\end{equation*}
We start with sampling from the three classes lying respectively on the three adjacent vertices of the regular hexagon. We gradually deteriorate the behavior of the dataset by sampling from the three remaining vertices in an anti-clockwise order. Further, from the $i^{th}$, class we sample $n_{i}$, number of points, where $n_{1}=5000$, $n_{2}=1500$, $n_{3}=4000$, $n_{4}=500$, $n_{5}=3500$, and $n_{6}=4500$.

\section{Description of datasets}
In Table \ref{classDesc} we give the details of the 12 selected higher-level classes alongside the leaf classes chosen for each of them. The Table \ref{datasetDesc} summarizes the properties (such as number of points, classes, IR, etc.) for each of the created datasets. Moreover, a dataset is named as ``D$CS$", where $C$ is the number of class and $S$ is a serial index. For example, $D101$ indicates the first 10-class dataset. 

\begin{table}[!ht]

  \begin{center}
    \caption{Selected Classes from ImageNet ILSVRC2012}
    \label{classDesc}
    \footnotesize
    \begin{tabular}{cccc} \toprule
      Selected & No. of & Leaf classes & ILSVRC2012  \\
      class (Serial$^*$) & Points & & Reference \\ \midrule
      \multirow{5}{*}{Animal (1)} & \multirow{5}{*}{6500} & Egyptian Cat & n02124075\\ 
      & & Cougar & n02125311\\ 
      & & Gazelle & n02423022\\ 
      & & Great Dane & n02109047\\ 
      & & Zebra & n02391049\\ \midrule
      \multirow{5}{*}{Artifact (2)} & \multirow{5}{*}{6394} & Revolver & n04086273 \\ 
      & & Desk & n03179701 \\ 
      & & Chainsaw & n03000684 \\ 
      & & Typewriter Keyboard & n04505470\\ 
      & & Teddy, Teddy Bear & n04399382 \\ \midrule
      \multirow{2}{*}{Dress (3)} & \multirow{2}{*}{2600} & Crash Helmet & n03127747 \\ 
      & & Gown & n03450230 \\ \midrule
      Factory (4) & 1300 & Lumber-mill & n03697007\\ \midrule
      \multirow{3}{*}{Food (5)} & \multirow{3}{*}{3900} & Strawberry & n07745940\\ 
      & & Mashed Potato & n07711569 \\ 
      & & Bagel & n07693725 \\ \midrule
      \multirow{3}{*}{Fungus (6)} & \multirow{3}{*}{3900}  & Hen-of-the-Woods & n13052670 \\ 
      & & Earthstar & n13044778 \\ 
      & & Stinkhorn & n13040303 \\ \midrule
      \multirow{4}{*}{Geological (7)} & \multirow{4}{*}{4200} & Cliff & n09246464\\ 
      & & Valley & n09468604\\ 
      & & Coral Reef & n09256479 \\ 
      & & Seashore & n09428293 \\  \midrule
      Natural (8) & 1300 & Rapeseed & n11879895\\ \midrule
      \multirow{2}{*}{Person (9)} & \multirow{2}{*}{2600} & Groom & n10148035 \\ 
      & & Scuba Diver & n10565667\\ \midrule
      \multirow{2}{*}{Plant (10)} & \multirow{2}{*}{2600} & Daisy & n11939491 \\ 
      & & Yellow lady slippers & n12057211 \\ \midrule
      \multirow{2}{*}{Sport (11)} & \multirow{2}{*}{2600} & Racket & n04039381 \\ 
      & & Barbell & n02790996 \\ \midrule
      \multirow{5}{*}{Vehicle (12)} & \multirow{5}{*}{6500} & Airliner & n02690373 \\ 
      & & Gondola & n03447447 \\ 
      & & Mountain Bike & n03792782\\ 
      & & Ambulance & n02701002\\ 
      & & Limousine & n03670208 \\ \bottomrule
      \multicolumn{4}{l}{$*$ The serial number will be hereafter used to represent the corresponding class.} \\ 
      \end{tabular}
  \end{center}
\end{table}

\begin{table}[t]
    \centering
    \caption{Properties of the datasets}
    \label{datasetDesc}
    \footnotesize
    \begin{tabular}{ccC{4cm}C{5cm}c} \toprule
    \scriptsize
        Dataset  & $C$ & Serial of  & Data points in  & $IR$ \\
        name &  & classes & each class & \\ \midrule
        D21 & 2 &1, 9 & \multirow{3}{*}{3000, 75} & \multirow{3}{*}{40} \\ 
        D22 & 2 & 12, 10 & & \\ 
        D23 & 2 & 2, 8 & & \\ \midrule
        D24 & 2 & 7, 4 & \multirow{3}{*}{3000, 150} & \multirow{3}{*}{20} \\ 
        D25 & 2 & 5, 11 & & \\ 
        D26 & 2 & 6, 3 & & \\ \midrule
        D27 & 2 & 1, 8 & \multirow{3}{*}{3000, 300} & \multirow{3}{*}{10} \\ 
        D28 & 2 & 12, 11 & & \\ 
        D29 & 2 & 6, 4& & \\ \midrule
        D210 & 2 & 7, 9 & \multirow{3}{*}{3000, 600} & \multirow{3}{*}{5} \\ 
        D211 & 2 & 2, 10 & & \\ 
        D212 & 2 & 5, 3 & & \\ \midrule
        D31 & 3 &1, 2, 8 & \multirow{4}{*}{2500, 1250, 100}& \multirow{4}{*}{25} \\  
        D32 & 3 &12, 10, 9 & & \\ 
        D33 & 3 &7, 5, 3 & & \\ 
        D34 & 3 &6, 11, 4 & & \\ \midrule
        D51 & 5 &1, 2, 4, 10, 5 & \multirow{3}{4cm}{\centering 3000, 1500, 750, 250, 100}& \multirow{3}{*}{30} \\ 
        D52 & 5 &7, 12, 9, 11, 3 & & \\ 
        D53 & 5 &6, 2, 9, 10, 8 & & \\ \midrule
        D101 & 10 & 1, 2, 5, 6, 7, 12, 10, 11, 4, 8 & \multirow{3}{4cm}{ \centering 2000, 1750, 1500, 1250, 1000, 750, 500, 250, 150, 100} & \multirow{3}{*}{20} \\  
        D102 & 10 & 1, 2, 5, 6, 12, 10, 11, 4, 9, 3 & & \\ 
        D103 & 10 & 1, 2, 6, 12, 10, 4, 9, 3, 7, 8 & & \\ \bottomrule
    \end{tabular}
\end{table}

\section{Parameter Setting of the classifiers used for empirical evaluation}
For Dual-LexiBoost all the parameters are set following the guidelines of the original article. To elaborate, in Dual-LexiBoost the $k$-nearest neighbor is chosen as the base classifier where the number of neighbors is set to 3; while the number of rounds is set to 10. For NBSVM, a linear kernel (using radial basis kernel did not significantly improve performance, possibly because Inception V3 induces linear separability among classes) is used while the regularization parameter is varied in the set $\{10, 100\}$. The number of iterations in RUSBoost is kept fixed at 10 while all the other parameters are set to the default as advised in the original article. The MLP is designed with one hidden layer containing $\sqrt{Cd}$ number of hidden nodes, while the parameters for SMOTE are set following the corresponding research article.

\end{document}
